# Supplementary material for: Broadband microwave spectroscopy of semiconductor nanowire-based Cooper-pair transistors
Source: arXiv:1901.10992 ancillary file (2020-03-04)
Supplement: Supplementary file 1 [file supplement.pdf]

**Supplementary Information**  
**Broadband microwave spectroscopy of semiconductor  
nanowire-based Cooper-pair transistors**

Alex Proutski,<sup>1,\*</sup> Dominique Laroche,<sup>1,\*</sup> Bas van 't Hooft,<sup>1</sup> Peter  
Krogstrup,<sup>2,3</sup> Jesper Nygård,<sup>3</sup> Leo P. Kouwenhoven,<sup>4,1</sup> and Attila Geresdi<sup>1,†</sup>

<sup>1</sup>*QuTech and Kavli Institute of Nanoscience,*

*Delft University of Technology, 2600 GA Delft, The Netherlands*

<sup>2</sup>*Microsoft Quantum Materials Lab Copenhagen, Niels Bohr Institute,*

*University of Copenhagen, 2100 Copenhagen, Denmark*

<sup>3</sup>*Center for Quantum Devices, Niels Bohr Institute,*

*University of Copenhagen, 2100 Copenhagen, Denmark*

<sup>4</sup>*Microsoft Quantum Lab Delft, 2600 GA Delft, The Netherlands*

(Dated: May 10, 2019)

---

\* These authors contributed equally to this work.

† Corresponding author; e-mail: a.geresdi@tudelft.nl

## I. DEVICE FABRICATION

The entire circuit is fabricated on top of an undoped Si wafer capped with a 285 nm thick thermally grown  $\text{SiO}_x$  layer. Each of the following fabrication step is defined using positive tone electron beam lithography. First, the electrostatic gates and the lower plane of the on-chip capacitors, made from Ti/Au (5/10 nm) using a conventional electron-beam evaporation tool, are deposited. Next, a 30 nm thick layer of  $\text{SiN}_x$  is sputtered to cover both of the metallic structures, forming an insulating barrier for the gates and capacitors. The resistive decoupling of the circuit is achieved through electron-beam evaporation of Cr/Pt (5/30 nm) with a net line resistivity, for a line width of 80 nm, of  $100 \Omega/\mu\text{m}$ . The lines are designed to fan out 120  $\mu\text{m}$  away from the circuit, leading to a total line resistance of 12 k $\Omega$ . In the following step, both tunnel junctions (the spectrometer and the reference SQUID junction) are created through the conventional Dolan-bridge angle evaporation technique, with the two layers being 9 and 11 nm thick, respectively. The tunnel barriers are created through an *in-situ* oxidation at 1.3 mbar for 4 minutes. The geometry of the devices is given in Table S1. The contact to the spectrometer junction is achieved through the electron-beam evaporation of Ti/Au (10/80 nm) after a 2 minute 30 seconds dry Ar etch to remove the native oxide. The upper layer of the on-chip capacitors were deposited simultaneously, creating coupling capacitance with  $C_C \approx 400$  fF. In the same step, the Ti/Au layer is also deposited on all but 28  $\mu\text{m}$  of the biasing lines of the spectrometer junction to reduce their resistance down to 2.8 k $\Omega$ .

The InAs nanowires with Al shell are then deterministically deposited on top of the gate pattern with the aid of a micro-manipulator setup. To define the junctions and the island in between, the Al layer is selectively removed from the desired region by performing a Transene D etch for 12 seconds at 48.2°C followed by a water rinse. In both devices, the channel length of the junctions is designed to be the same. The epitaxial Al layer is approximately 5 nm thick for both devices, and was grown on two facets. The contacts to the nanowire and the reference SQUID junction are achieved through sputtering a 120 nm layer of NbTiN with a 2 minute Ar plasma milling performed beforehand. Design parameters of both devices are given in Table S1.

|                                                  | Device 1         | Device 2         |
|--------------------------------------------------|------------------|------------------|
| Channel length (nm)                              | 100              | 100              |
| Island length ( $\mu\text{m}$ )                  | 0.8              | 1.75             |
| Reference tunnel junction area ( $\text{nm}^2$ ) | $750 \times 100$ | $750 \times 100$ |
| SQUID periodicity ( $\mu\text{T}$ )              | 100              | 100              |
| Spectrometer junction area ( $\text{nm}^2$ )     | $100 \times 100$ | $100 \times 100$ |

TABLE S1. Geometry of the circuit components.

## II. MEASUREMENT SETUP

The measurements were performed in a Leiden Cryogenics CF-1200 dry dilution refrigerator with a base temperature of  $\approx 18\text{ mK}$ . The electrical connections to the sample were established via Cu/Ni twisted pair cables thermally anchored at all stages of the refrigerator to ensure good thermalization. To suppress any external noise, each line was filtered first at room temperature by  $\pi$ -LC filters (cutoff  $\approx 100\text{ MHz}$ ) and at base temperature by copper-powder (cutoff  $\approx 1\text{ GHz}$ ) and RC (cutoff  $\approx 50\text{ kHz}$ ) filters. The spectrometer was probed under DC bias in a 4 point geometry (device 1) or a 3 point geometry (device 2). In the 3 point geometry, a series resistance of  $3088\ \Omega$  was subtracted from the raw  $I(V)$  curve.

## III. CIRCUIT PARAMETERS

For both devices, the circuit was analysed through the observation of the plasma peak in the  $I(V)$  response of the spectrometer with both junctions of the nanowire in full depletion. We insert the impedance  $\text{Re}[Z(\omega)]$  into Eq. (1) in the main text as:

$$\text{Re}[Z(x)] = \frac{Z_0 Q}{1 + \frac{Q^2}{x^2} (1 - x^2)^2} \quad (\text{S1})$$

Here  $Q = R\sqrt{C/L}$  is the quality factor and  $Z_0 = \sqrt{L/C}$  is the characteristic impedance of the circuit. We introduced a dimensionless frequency  $x = \omega/\omega_0$  defined with  $\omega_0 = 1/\sqrt{LC}$ . We display the obtained fits of Eq. (S1) in Fig. S1. We attribute the deviation between the fits and data at higher frequencies to additional losses or modes not accounted for by Eqs. (1) and (S1).

From measurements of the superconducting gap and the normal state resistance acquired

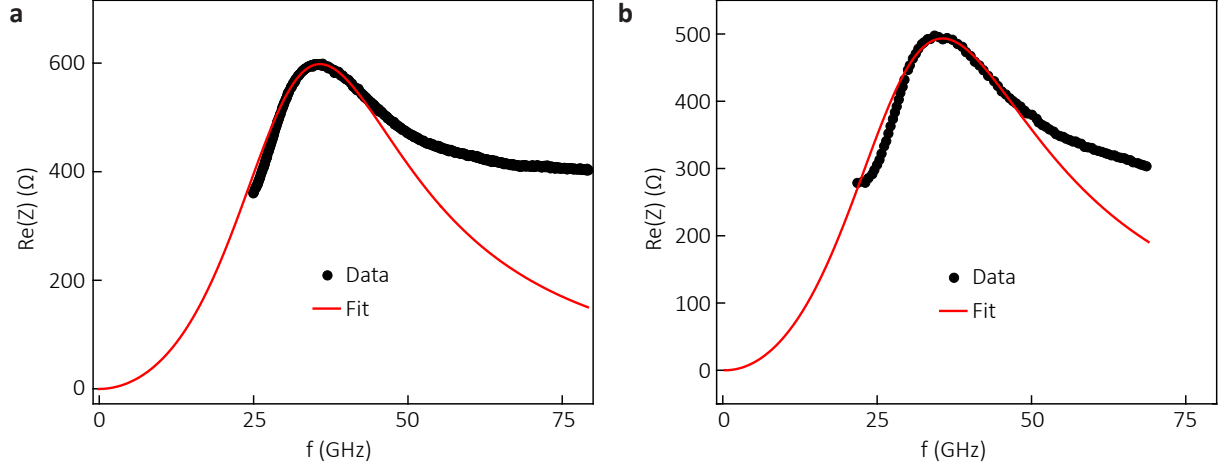

FIG. S1. Fit to the plasma resonance of the circuit. The measured data is represented by black dots with the fit based on Eq. (S1) shown as a red line for device 1 (a) and device 2 (b), respectively.

at voltage biases much higher than the gap at low temperatures, we determine the Josephson energy  $E_J$  and the Josephson inductance  $L_J$  of each tunnel junction. This allows us to determine all of the relevant circuit parameters, listed in Table S2.

|                                                                                                            | Device 1         | Device 2          |
|------------------------------------------------------------------------------------------------------------|------------------|-------------------|
| Tunnel junction resistance $R_J$ (k $\Omega$ )                                                             | 3.17             | 2.96              |
| Tunnel junction gap $\Delta_J$ ( $\mu$ eV)                                                                 | 245              | 245               |
| Tunnel junction critical current $I_{c,J} = \frac{\pi\Delta_J}{2eR_J}$ (nA)                                | 121.4            | 130.3             |
| $E_{JL} = \frac{\hbar I_{c,J}}{2e}$ ( $\mu$ eV)                                                            | 249              | 267.3             |
| Tunnel junction inductance $L_J = \frac{\Phi_0}{2\pi I_{c,JJ}}$ (nH)                                       | 2.71             | 2.53              |
| Spectrometer resistance $R_{\text{spec}}$ (k $\Omega$ )                                                    | 14.44            | 12.7              |
| Spectrometer gap $\Delta_{\text{spec}}$ ( $\mu$ eV)                                                        | 238              | 241               |
| Spectrometer critical current $I_{c,\text{spec}} = \frac{\pi\Delta_{\text{spec}}}{2eR_{\text{spec}}}$ (nA) | 25.9             | 30.3              |
| Shunt resistance $R$ ( $\Omega$ )                                                                          | $598.1 \pm 0.3$  | $493.3 \pm 0.87$  |
| Shunt capacitance $C_L$ (fF)                                                                               | $7.28 \pm 0.01$  | $8.04 \pm 0.03$   |
| Charging energy $E_{CL} = \frac{2e^2}{C_L}$ ( $\mu$ eV)                                                    | $43.96 \pm 0.07$ | $39.8 \pm 0.15$   |
| Plasma frequency $f_p = \frac{1}{2\pi\sqrt{L_J C_L}}$ (GHz)                                                | $35.83 \pm 0.02$ | $35.29 \pm 0.07$  |
| Characteristic impedance $Z_0 = \sqrt{\frac{L_J}{C_L}}$ ( $\Omega$ )                                       | $610.1 \pm 0.42$ | $561.0 \pm 1.05$  |
| Quality factor $Q = R\sqrt{\frac{C_L}{L_J}}$                                                               | $0.98 \pm 0.001$ | $0.88 \pm 0.0025$ |

TABLE S2. Circuit parameters of the devices featured in the current study.

#### IV. SPECTRUM ANALYSIS

The excitation energies of the circuit reveal themselves as peaks in the measured  $I(V)$  traces of the spectrometer. We are interested in discerning the modes that arise due to the nanowire CPT which manifest themselves as additional peaks observed on top of the plasma mode. In order to improve their visibility we evaluate  $|d\text{Re}[Z(\omega)]/dV_{\text{spec}}|$  after applying a Gaussian low pass filter (Fig. S2). Transitions superimposed on the plasma mode peak appear as minima in  $|d\text{Re}[Z(\omega)]/dV_{\text{spec}}|$ .

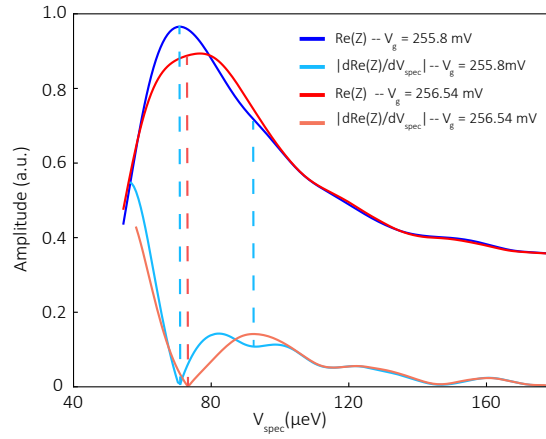

FIG. S2. Analysis of the measured  $I_{\text{spec}}(V_{\text{spec}})$ . The blue and red lines represent  $\text{Re}(Z)(V_{\text{spec}})$  for device 1 obtained at two  $V_g$  values. The light blue and orange lines display  $|d\text{Re}[Z(\omega)]/dV_{\text{spec}}|$  with the dashed line indicating the position of the resonances arising due to the nanowire CPT and the hybrid SQUID.

## V. THEORY

We establish the hybrid SQUID Hamiltonian based on the circuit shown in Fig. 2a. We associate a voltage with each node and write the charging energy of the system as

$$T = \frac{1}{2}C_L(V_1 - V_2)^2 + \frac{1}{2}C_1(V_1 - v)^2 + \frac{1}{2}C_2(v - V_2)^2 + \frac{1}{2}C_G(V_1^2 + V_2^2) + \frac{1}{2}C_{ig}(v - V_g)^2. \quad (\text{S2})$$

Similarly, the total Josephson energy is as follows:

$$U = -E_{J1} \cos(\varphi_1) - E_{J2} \cos(\varphi_2) - E_{JL} \cos(\varphi - \varphi_1 - \varphi_2). \quad (\text{S3})$$

Now we obtain the Lagrangian of the system as:

$$\mathcal{L} = T - U, \quad (\text{S4})$$

and use the phase  $\varphi_n$  and charge  $q_n$  as the canonical conjugate variables:

$$q_n = \frac{\partial \mathcal{L}}{\partial \dot{\varphi}_n} \text{ and } \phi_n = \frac{\partial \mathcal{L}}{\partial \dot{q}_n}. \quad (\text{S5})$$

Note that each voltage difference in Eq. (S2) can be expressed with the phase  $V = \varphi_0 \dot{\varphi}$ , where  $\varphi_0 = \Phi_0/2\pi$  is the reduced flux quantum. Next, we obtain the Hamiltonian of the circuit:

$$H = \Sigma_i \dot{\varphi}_i \frac{\partial \mathcal{L}}{\partial \dot{\varphi}_i} - \mathcal{L}, \quad (\text{S6})$$

which we can express in the following form:

$$H = \frac{1}{2} \frac{(q_1 - q_g)^2}{C_{Det}^2/C_{i2}} + \frac{1}{2} \frac{(q_2 + q_g)^2}{C_{Det}^2/C_{i1}} - \frac{(q_1 - q_g)(q_2 + q_g)}{C_{det}^2/C_{ic}} + U, \quad (\text{S7})$$

where  $q_g = C_{ig}V_g/(2 + C_{ig}/C_G)$  and

$$C_{i1} = C_L + C_1 + \frac{(1 + \frac{C_{ig}}{C_G})^2 C_G + C_G + C_{ig}}{(2 + \frac{C_{ig}}{C_G})^2} \quad (\text{S8})$$

$$C_{i2} = C_L + C_2 + \frac{(1 + \frac{C_{ig}}{C_G})^2 C_G + C_G + C_{ig}}{(2 + \frac{C_{ig}}{C_G})^2} \quad (\text{S9})$$

$$C_{ic} = C_L + \frac{C_G}{2 + \frac{C_{ig}}{C_G}} \quad (\text{S10})$$

$$C_{Det}^2 = C_{i1}C_{i2} - C_{ic}^2. \quad (\text{S11})$$

Finally, we write the Hamiltonian operator with the conjugate number and phase operators, which pairwise obey  $[\hat{\varphi}_{1,2}, \hat{N}_{1,2}] = i$ :

$$\begin{aligned} \hat{H} = & \frac{1}{2}E_{C1}(\hat{N}_1 - n_g)^2 + \frac{1}{2}E_{C2}(\hat{N}_2 + n_g)^2 - \frac{1}{2}E_{Cc}(\hat{N}_1 - n_g)(\hat{N}_2 + n_g) \\ & - E_{J1} \cos(\hat{\varphi}_1) - E_{J2} \cos(\hat{\varphi}_2) - E_{JL} \cos(\varphi - \hat{\varphi}_1 - \hat{\varphi}_2) \end{aligned} \quad (\text{S12})$$

With a set of effective charging energies defined as:

$$E_{C1} = (2e)^2 C_{i2} / C_{Det}^2 \quad (\text{S13})$$

$$E_{C2} = (2e)^2 C_{i1} / C_{Det}^2 \quad (\text{S14})$$

$$E_{Cc} = (2e)^2 C_{ic} / C_{Det}^2. \quad (\text{S15})$$

We diagonalize  $\hat{H}$  in the charge basis, span by  $N_1$  and  $N_2$ , where the Josephson terms act as stepping operators,  $e^{\pm i\hat{\varphi}_i} |N_i\rangle = |N_i \pm 1\rangle$ .

## VI. METHODS

### A. Model size

The eigenvectors and eigenvalues for the system at every gate charge value between -1 and 1 are numerically computed with a maximal value of  $N_i = \pm 4$ . This value has to be sufficiently large to ensure that the wavefunctions have negligible weight near the extremum values of  $N_i$ . As shown in Fig. S3, the extracted eigenenergies of the system for typical energy scales do not change if the system size is further increased.

### B. Peak extraction

First, all minimum values in  $|d\text{Re}(Z)/dV_{\text{spec}}|$  are collected, using both  $V_g$  and  $V_{\text{spec}}$  line-cuts. Then, using  $E_{JL}$  extracted from the bare SQUID IV trace and initial guesses for  $E_{C1}, E_{C2}, E_{Cc}, E_{J1}$  and  $E_{J2}$ , a first iteration of the dispersion relation of the CPT is calculated from the model described in the previous section. It is important that this initial guess yields a good visual agreement between the calculated dispersion relation and the

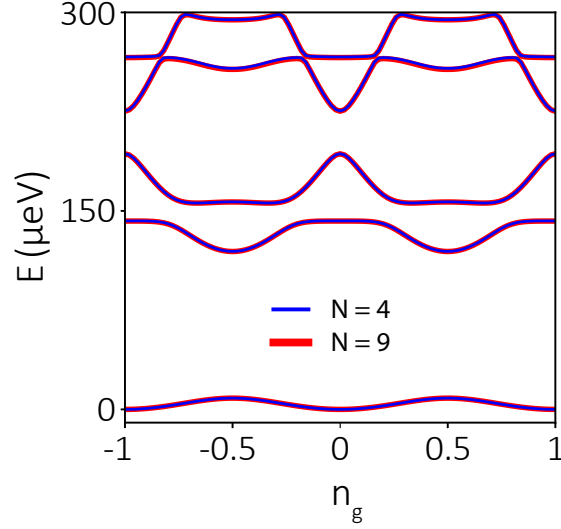

FIG. S3. The calculated energy levels as a function of  $n_g$  at  $\varphi = \pi$  of the hybrid SQUID using  $N = 4$  and  $N = 9$  for  $E_{C1} = 168 \mu\text{eV}$ ,  $E_{C2} = 260 \mu\text{eV}$ ,  $E_{Cc} = 188 \mu\text{eV}$ ,  $E_{J1} = 132 \mu\text{eV}$ ,  $E_{J2} = 16 \mu\text{eV}$  and  $E_{JL} = 249 \mu\text{eV}$ .

experimentally observed features in the measured data. Then, at each experimental gate charge and for each energy mode, the closest minima to this first estimate is used as the experimental dispersion relation.

This method was used to extract the experimental dispersion relation of all data sets in this article except for the data of Fig. 3e. In this case, due to the flat dispersion relation of both the plasma and the CPT modes in gate space, minima in  $|d^2\text{Re}(Z)/dV_{\text{spec}}^2|$  are used to identify features in  $\text{Re}[Z(\omega)]$ . To ensure that the right features were tracked in this manner, the expected position of the features is inferred from a separate data set (Fig. 3f) showing the phase dependence of  $\text{Re}[Z(\omega)]$ .

### C. Fitting procedure

To determine the charging and Josephson energies of the hybrid system, a least-square minimization was performed on the difference between experimental data points and the calculated excitation spectra. This minimization was performed on the two lowest excitation energies for both a gate charge scan (eg. Fig. S4a) and a flux scan (eg. Fig. S4b) simultaneously. The least-square minimization was performed on 2 periods in gate space (range

$4e$ ) and 1 period in flux space (range  $2\pi$ ). The minimization procedure was carried out iteratively by varying the set  $E_{C1}, E_{C2}, E_{Cc}, E_{J1}, E_{J2}$  through  $\sim 60000$  combinations while keeping  $E_{JL}$  fixed at the value determined from the plasma mode fit (see Table. S2). The first iteration started from an initial guess and typically spanned over a range of  $\pm 40 \mu\text{eV}$  for  $E_{C1}$  and  $E_{C2}$  and  $\pm 30 \mu\text{eV}$  for  $E_{J1}$ .  $E_{Cc}$  was varied as a fraction of the geometrical mean of  $E_{C1}$  and  $E_{C2}$ , typically  $0.87 \pm 0.09$ , and  $E_{J2}$  was varied as a fraction of  $E_{J1}$ , typically  $0.25 \pm 0.1$ . This process iterated around the previous optimal value with progressively smaller parameter range until the optimal energies were changing by less than  $4 \mu\text{eV}$ . The procedure was performed over a few different initial guesses, and it was verified that the solutions converged to the same set of parameters.

#### D. Even-odd occupation

After interpolation and applying a Gaussian filter to the measured spectra, a linecut, corresponding to a gate voltage value halfway between the odd and the even peaks, was subtracted. To account for the background of our data, another linecut, corresponding to a large  $V_{\text{spec}}$  away from resonances, was subtracted. Following this, the spectrometer voltage value  $V_{\text{spec}}^{\text{max}}$  for the maximum  $\delta I_{\text{spec}}$  current oscillations was selected, and we find  $2eV_{\text{spec}}^{\text{max}} \approx 180 \mu\text{eV}$  for Fig. 4 and  $2eV_{\text{spec}}^{\text{max}} \approx 240 \mu\text{eV}$  for Fig. S6. The large and small current peaks are attributed to the even and odd occupation, respectively. Finally, the current values  $\delta I_{\text{even}}$  and  $\delta I_{\text{odd}}$  were averaged over 3 data points in  $V_{\text{spec}}$  (centered about  $V_{\text{spec}}^{\text{max}}$ ) and over 3 data points in gate voltage (centered about the peaks) for each peak. Assuming that the current response is proportional to the initial occupation probability, we can write  $p_{\text{even}} = \delta I_{\text{even}} / (\delta I_{\text{even}} + \delta I_{\text{odd}}) = (1 + \delta I_{\text{odd}} / \delta I_{\text{even}})^{-1}$ .

## VII. ADDITIONAL DATASETS

### A. Theoretical description of measured spectra

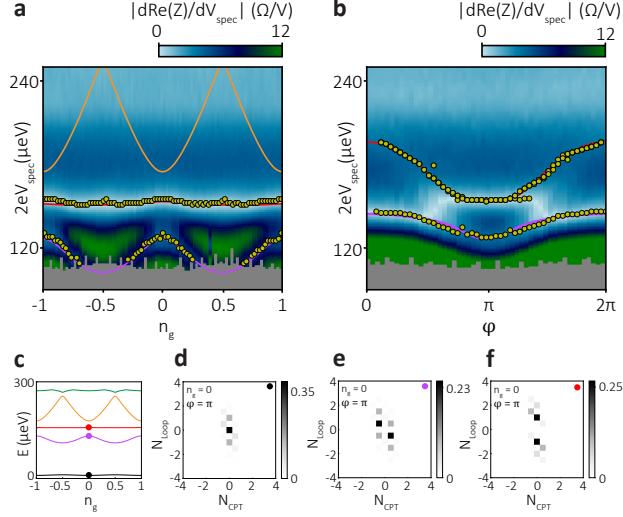

FIG. S4. The observed transitions for device 1 as a function of the gate charge,  $n_g$  (a) and applied phase bias  $\varphi = 2\pi\Phi/\Phi_0$  (b). The transitions are identified at the local minima of  $|d\text{Re}(Z)/dV_{\text{spec}}|$  (yellow dots). The best fit is shown with solid lines, yielding  $E_{C1} = 93 \mu\text{eV}$ ,  $E_{C2} = 184 \mu\text{eV}$ ,  $E_{Cc} = 104 \mu\text{eV}$ ,  $E_{J1} = 148 \mu\text{eV}$ ,  $E_{J2} = 46 \mu\text{eV}$ . (c) The corresponding energy bands of the device as a function of  $n_g$  at  $\varphi = \pi$ . The two component probability distributions of the ground state (d), first excited state (e) and second excited state (f) at  $n_g = 0$  and  $\varphi = \pi$ , denoted by circles of the corresponding colour in panel (c). Here,  $V_{t1} = 0.4 \text{ V}$ ,  $V_{t2} = 1.92 \text{ V}$ , and  $V_g = 713.1 \dots 719.7 \text{ mV}$ .

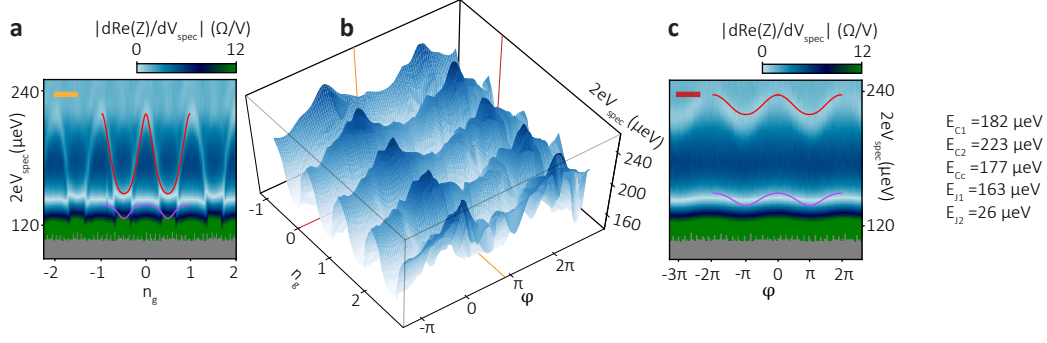

FIG. S5. The measured excitations spectrum of device 1 as a function of  $n_g$  and  $\varphi$  with  $V_{tg1} = 0.55 \text{ V}$ ,  $V_{tg2} = 0.9 \text{ V}$  and  $V_g = 250 \dots 264.5 \text{ mV}$ . Panel (b) shows the full map of the second excitation, whereas the linecuts are shown in panels (a) and (c) at the positions denoted by the orange and red lines, respectively. The best fits of the first two excitations energies are overlain in panels (a) and (c). The data was taken on device 1 and the parameters of the best fit are listed on the right.

## B. Temperature dependence

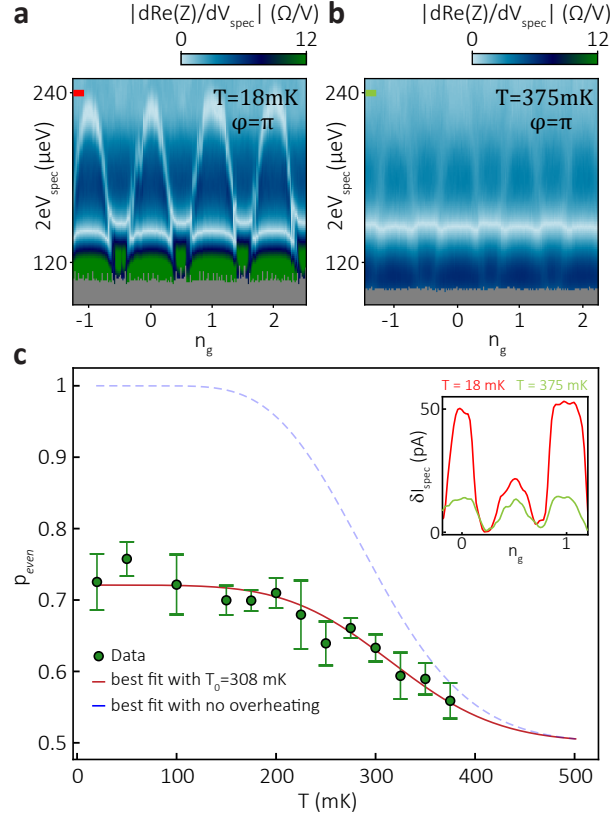

FIG. S6. The measured spectra of device 1 at  $V_{\text{tg}1} = 2.1 \text{ V}$ ,  $V_{\text{tg}2} = 2.43 \text{ V}$  and  $V_g = -536 \dots -521.5 \text{ mV}$  as a function of  $n_g$  at  $\varphi = \pi$  and at a temperature of 18 mK (a) and 375 mK (b). (c) The extracted even charge parity state occupation as a function of temperature saturating at  $p_{\text{even}} \approx 0.72$ . The inset shows the modulation of the spectrometer current at  $2eV_{\text{spec}} = 240 \mu\text{eV}$  at these two temperatures which defines  $\delta I_{\text{odd}}$  and  $\delta I_{\text{even}}$ . The fit lines in (c) are without (blue dashed line) and including (red solid line) overheating, respectively. The fit yields  $T_0 = 308 \pm 6 \text{ mK}$ ,  $V = 4.94 \times 10^{-24} \text{ m}^{-3}$ ,  $\Delta = 97 \pm 3 \mu\text{eV}$  and  $n_{qp} \approx 3 \times 10^4 \mu\text{m}^{-3}$ .
